# Supplementary material for: Sensitive particle shape dependence of growth-induced mesoscale nematic structure
Source: arXiv:2501.15681 ancillary file (2025-01-30)
Supplement: Supplementary file 1 [file supplement.pdf]

# Supplementary Information for Sensitive particle shape dependence of growth-induced mesoscale nematic structure

Jonas Isensee and Philip Bittihn*

*Department of Living Matter Physics, Max Planck Institute for Dynamics and Self-Organization, Göttingen, Germany and Institute for Dynamics of Complex Systems, University of Göttingen, Göttingen, Germany*

* philip.bittihn@ds.mpg.de

## I. MODEL DEFINITIONS

Pairwise interactions in the regular rod model are defined using line segments connecting the two half-circle caps within each rod as illustrated in Fig. 1. The important observation is that the shape of such a rod is fully defined by a line segment and an associated radius $R$. From these, one can efficiently compute the pair of closest points on the segments connected by vector $\mathbf{d}$ and use those to define the repulsion force as

$$\mathbf{F}(\mathbf{d}) = \begin{cases} \frac{Y}{2}\sqrt{\frac{R}{2}}\,(2R - |\mathbf{d}|)^{\frac{3}{2}}\,\hat{\mathbf{d}}, & |\mathbf{d}| \leq 2R \\ 0, & |\mathbf{d}| > 2R \end{cases}$$

with with hardness pre-factor $Y$ and further details in [1].

The agents are constructed using an internal frame of line segments as illustrated in Fig. 2. For pointiness values $\mathcal{P} \leq 1$ the frame forms a rectangle and for values greater than $\mathcal{P} \geq 1$ it gains the triangle tips. The agent shapes are parameterized by bounding box area, aspect and pointiness, and therefore the precise frame shape and pseudo-radius are computed to conform to that:

| | |
|---|---|
| bounding box area | $A = 2$ |
| division aspect | $a_\mathrm{d}$ |
| width | $w = \sqrt{A/a_\mathrm{d}}$ |
| (division) length | $l_\mathrm{max} = \sqrt{A a_\mathrm{d}}$ |
| pointiness | $\mathcal{P}$ |
| pseudo radius | $r_p = (1 - \lvert\mathcal{P} - 1\rvert)w/2$ |
| frame width | $w - 2r_p$ |
| frame length | $l - 2r_p$ |

For pointiness approaching $\mathcal{P} \to 1$ from both sides, the respective frame shapes collapse onto a single line and recover the original rod in good approximation (See Section II).

As a response to net-forces $\mathbf{f}$ and torque $\tau$, agents move on the substrate according to

$$\mathbf{v} = \mu_\mathrm{tr}\mathbf{f}$$

$$\partial_t \phi = \mu_\mathrm{r}\tau$$

with velocity $\mathbf{v}$, orientation $\phi$, and (isotropic) translational and rotational mobility $\mu$. These

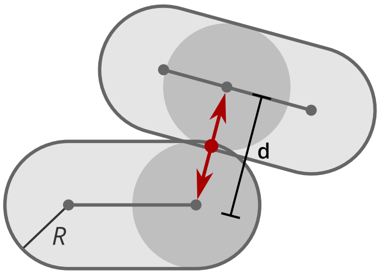


**Figure 1:** Illustration of repulsion force computation for regular rod-like cells.

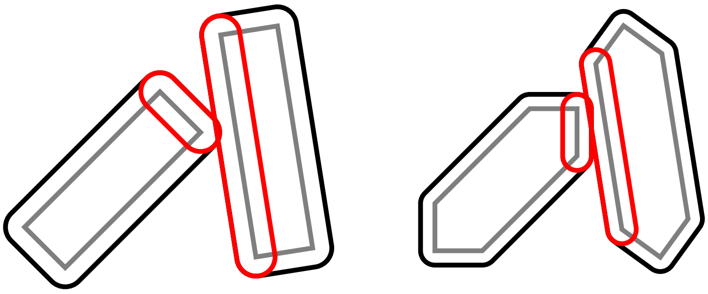

**Figure 2:** Illustration of how a frame of rod-like line segments is used to build the interaction function of the rod-derived models.

are defined as

$$\mu_{\text{trans}} = \frac{\mu_0}{wl}$$
$$\mu_{\text{rot}} = \frac{12}{w^2 + l^2}\mu_{\text{trans}}$$

using isotropic friction for area elements and integrating over the co-rotated bounding box $(w, l)$.

## II. CONVERGENCE OF STATISTICS FOR APPROXIMATE RODS

As mentioned in Section I, the concrete implementations of the rod-derived models differ for pointiness values greater and smaller than one. Both versions can also emulate the limiting case of the regular rod at pointiness 1.

To check consistency of the implementations a set of simulations with division aspect 2 was done for varied pointiness $\mathcal{P} \approx 1$. The relative angles of pairwise interactions between agents are gathered into probability distributions and displayed in Fig. 3. We find these

to depend sensitively on the pointiness $\mathcal{P}$ but still transition smoothly from one model implementation to the other at $\mathcal{P} = 1$.

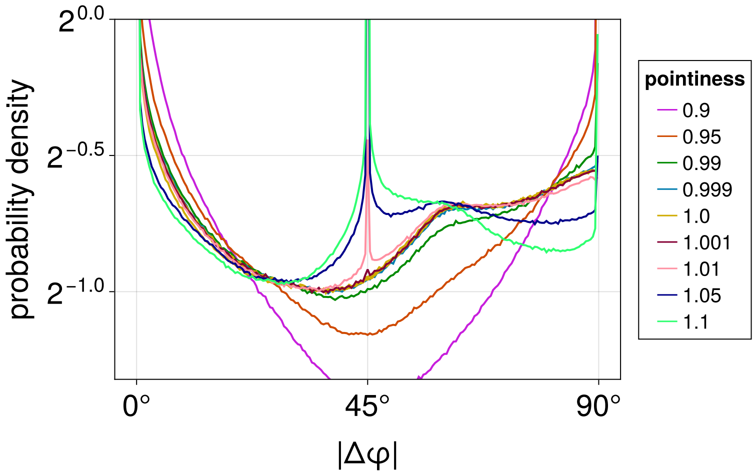


**Figure 3:** Pairwise orientation statistics have a well-defined limiting behaviour as the pointiness approaches unity from both sides.

### A. Supplementary Figures

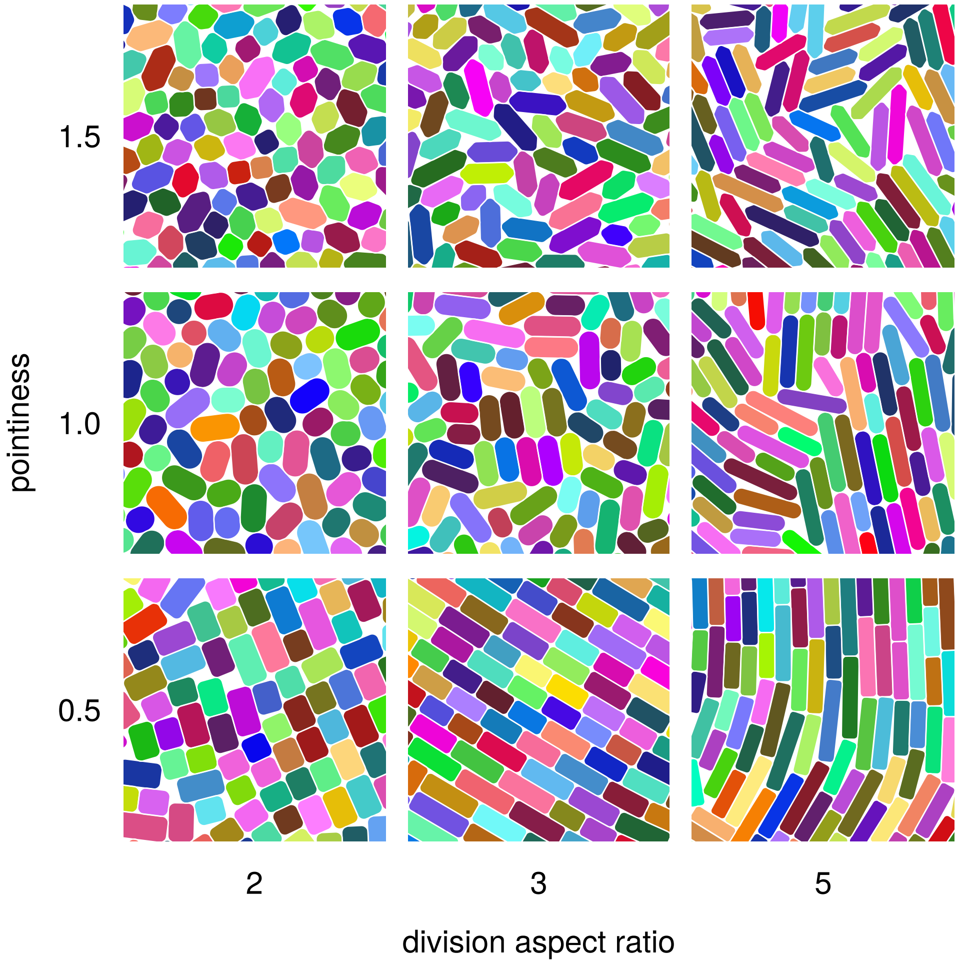


**Figure 4:** Typical arrangements of cells of varied shape and aspect ratio.

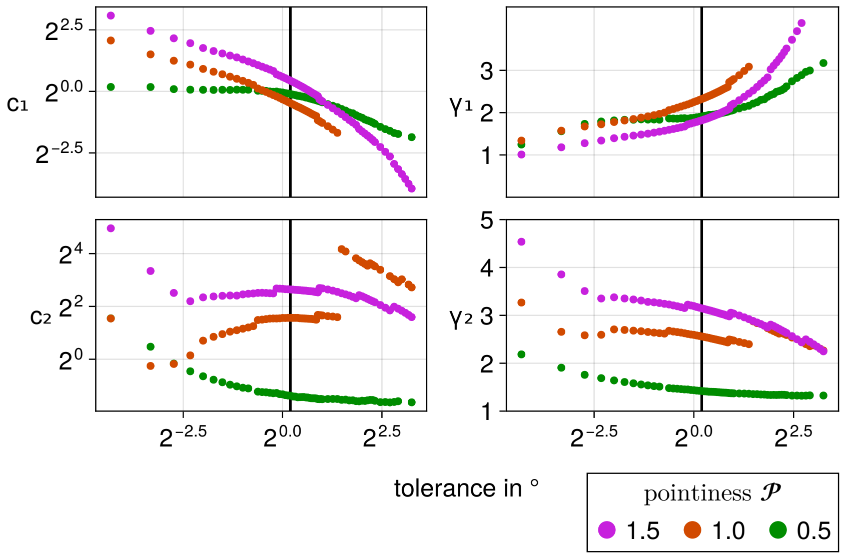


**Figure 5:** Fit parameters of main text Eq. (1) to distributions from simulations with varied parameters (see legend) as a function of clustering tolerance. The tolerance used in the main text analysis is indicated using a vertical line.


[1] J. Isensee, L. Hupe, R. Golestanian, and P. Bittihn, J. R. Soc. Interface **19**, 20220512 (2022).
